# Supplementary material for: Multi-Facet Blending for Faceted Query-by-Example Retrieval
Source: arXiv:2412.01443 source file (2024-12-02)
Supplement: Supplementary file 1 [file appendix.tex]

\appendix

\appendix
